# Supplementary material for: UADet: A Remarkably Simple Yet Effective Uncertainty-Aware Open-Set Object Detection Framework
Source: arXiv:2412.09229 source file (2024-12-12)
Supplement: Supplementary file 1 [file 7_appendix.tex]

\setcounter{table}{0}

\setcounter{figure}{0}

\section{More Experimental Details}

\subsection{Datasets}
In this section, we introduce more details about the dataset construction.

\noindent {\bf PASCAL VOC~\cite{everingham2010pascal}.} We use VOC07 \texttt{train} and VOC12 \texttt{trainval} splits for the training, and VOC07 \texttt{test} split to evaluate the close-set performance.
We take VOC07 \texttt{val} as the validation set.

\noindent {\bf VOC-COCO-T$_1$.} We divide 80 COCO classes into four groups (20 classes per group) by their semantics~\cite{joseph2021towards}: 
{\bf (1)} VOC classes. {\bf (2)} Outdoor, Accessories, Appliance, Truck. {\bf (3)} Sports, Food. {\bf (4)} Electronic, Indoor, Kitchen, Furniture.
We construct VOC-COCO-\{20, 40, 60\} with $n$=5000 VOC testing images and \{$n$, 2$n$, 3$n$\} COCO images {\bf containing} \{20, 40, 60\} non-VOC classes with semantic shifts, respectively.
Note that we only ensure each COCO image contains objects of corresponding open-set classes, which means objects of VOC classes will also appear in these images.
This setting is more similar to real-world scenarios where detectors need to carefully identify unknown objects and do not classify known objects into the unknown class.

\noindent {\bf VOC-COCO-T$_2$.} We gradually increase the Wilderness Ratio to build four dataset with $n$=5000 VOC testing images and \{0.5$n$, $n$, 2$n$, 4$n$\} COCO images {\bf disjointing} with VOC classes.
Compared with the setting {\bf T$_1$}, {\bf T$_2$} aims to evaluate the model under a higher wilderness, where large amounts of testing instances are not seen in the training.

\noindent {\bf Comparisons with existing benchmarks.}
\cite{dhamija2020overlooked} proposed the first OSOD benchmark. They also use the data in VOC for close-set training, and both VOC and COCO for open-set testing. In the testing phase, they just vary the number of open-set images sampled from COCO, while ignoring the number of open-set categories.
~\cite{joseph2021towards} proposed an open world object detection benchmark. They divide the open-set testing set into several groups by category. However, the wilderness ratio of each group is limited, and such data partitioning cannot reflect the real performance of detectors under extreme open-set conditions.
In contrast, our proposed benchmark considers both the number of open-set classes (VOC-COCO-T$_1$) and images (VOC-COCO-T$_2$).

On the other hand, some works on open-set panoptic segmentation~\cite{hwang2021exemplar} divide a single dataset into close-set and open-set. If a image contains both close-set and open-set instances, they just remove the annotations of open-set instances.
Differently, we strictly follows the definition in OSR~\cite{scheirer2012toward} that unknown instances should not appear in training.
To acquire enough open-set examples, we take both VOC and COCO from cross-dataset evaluation, which is a common practice in OSR~\cite{kong2021opengan,sun2020conditional,zhou2021learning}.

\subsection{Implementation Details}
% Hyper-parameter settings, training schedules.
% extend to one-stage detector
\noindent {\bf Training schedule.} Inspired by~\cite{vaze2021open} that a good close-set classifier benefits OSR, we train all models with the 3$\times$ schedule (\emph{i.e.}, 36 epochs). 
Besides, we enable UPL after several warmup iterations (\emph{e.g.}, 100 iterations) to make sure the model produce valid probabilities.

\noindent {\bf Open-RetinaNet.} We change some hyper-parameters for Open-RetinaNet.
In OpenDet, we take object proposals as examples and apply CFL to proposal-wise embeddings, which are equivalent to the anchor boxes in RetinaNet.
Therefore, we optimize Instance Contrastive Loss $\mathcal{L}_{IC}$ with pixel-wise features of each anchor box.
Since the number of anchor box is much larger than the proposals in OpenDet, we enlarge the memory size $Q$=1024, sampling size $q$=64, and loss weight to 0.2 in CFL.
Similar, we sample 10 hard examples rather than 3 in UPL.

\subsection{Evaluation Metrics}
% WI definition
% APU calculation
Firstly, we give a detailed formulation of the Wilderness Impact~\cite{dhamija2020overlooked}, which is defined as:
\begin{equation}
\begin{aligned}
    WI &= \frac{P_\mathcal{K}}{P_\mathcal{K \cup U}} - 1  \\
       &=  \frac{TP_\mathcal{K}}{TP_\mathcal{K}+FP_\mathcal{K}} / \frac{TP_\mathcal{K}}{TP_\mathcal{K}+FP_\mathcal{K}+FP_\mathcal{U}}  - 1 \\
       &= \frac{FP_\mathcal{U}}{TP_\mathcal{K}+FP_\mathcal{K}},
\end{aligned}
\end{equation}
where $FP_\mathcal{U}$ means that any detections belonging to the unknown classes $C_\mathcal{U}$ are classified to one of known classes $C_\mathcal{K}$.
For \APU~(AP of unknown classes), we merge the annotations of all unknown classes into one class, and calculate the \emph{class-agnostic} AP between unknown's predictions and the ground truth.

\section{Additional Main Results}
Due to limited space in our main paper, we report the results on VOC-COCO-2$n$ in Tab.~\ref{tab:voc_coco_2n}, where OpenDet shows significant improves than other methods.

% VOC-COCO-2n
\begin{table}[h]
    \input{tables/appendix/voc_coco_2n.tex}
    \caption{{\bf Comparisons with other methods on VOC-COCO-2$n$.}
    This table is an extension of Tab.2 in our main paper.
    }
    % \vspace{-3mm}
    \label{tab:voc_coco_2n}
    \end{table}

\section{Additional Ablation Studies}

\begin{figure}[t]
    \includegraphics[width=\linewidth]{figures/appendix/wp.pdf}
    \vspace{-3mm}
    \caption{{\bf Visualization of different $w(\cdot)$.}}
    \label{fig:plot_wup}
\end{figure}
    
\begin{table}[t]
    \input{tables/appendix/region_expanding.tex}
    \caption{{\bf Quantitative analyses of the latent space.} We calculate the intra-class variance and inter-class distance of latent features.}
    \label{tab:region_expanding}
\end{table}

\begin{table}[t]
    \input{tables/appendix/cfl_loss_weight.tex}
    \vspace{-3mm}
    \caption{{\bf Loss weight of $\mathcal{L}_{IC}$.} \emph{w/o} decay: $\gamma_t$ is a constant (\emph{i.e.}, 0.1) instead of variable.}
    \label{tab:weight_cfl}
    \end{table}

\begin{table}[t]
    \input{tables/appendix/cfl_temperature.tex}
    \caption{{\bf Temperature $\tau$ in $\mathcal{L}_{IC}$.}}
    \label{tab:tau_cfl}
    \end{table}

\noindent {\bf Visual analyses of $w(\cdot)$.} 
In Fig.~\ref{fig:plot_wup}, we plot the graph of different $w(\cdot)$.
Compared with entropy: $-p\log(p)$, the proposed function $(1-p)^\alpha \cdot p$ can adjsut the curve shape by changing $\alpha$.
In other words, the model adjusts the weights of examples as $\alpha$ changes.
The right of Fig.~\ref{fig:plot_wup} reports the model's open-set performance by varying $\alpha$, where smaller $\alpha$ reduces WI and AOSE.

\noindent {\bf Quantitative analyses of latent space.}
In Fig.~\ref{fig:tsne_vis} of the main paper, we give a visual analyses of latent space. Here we give a quantitative analyses of latent space in Tab.~\ref{tab:region_expanding}.
Specifically, we calculate the intra-class variance and inter-class distance of latent features.
Tab.~\ref{tab:region_expanding} shows that CFL and UPL, as well as their combination reduce intra-class variance and enlarge inter-class distance.
The results further confirm our conclusion in the main paper that our method can expand low-density latent regions.

\noindent {\bf More hyper-parameters in CFL.}
{\bf Loss weight:} Tab.~\ref{tab:weight_cfl} shows that loss weight is important for $\mathcal{L}_{IC}$, where a small weight (\emph{e.g.}, 0.01) cannot learn compact features and a large weight (\emph{e.g.}, 1.0) hinder the generalization ability.
Besides, Tab.~\ref{tab:weight_cfl} (last column) also demonstrates the effectiveness of loss decay.
{\bf Temperature:} We try different $\tau$ that used in pervious works~\cite{he2020momentum,khosla2020supervised}.
Tab.~\ref{tab:tau_cfl} indicates that $\tau$=0.1~\cite{khosla2020supervised} works better than other settings.

\noindent {\bf Training strategy.}
Some works in OSR~\cite{zhou2021learning} adopted a pretrain-then-finetune paradigm to train the unknown identifier.
We carefully design the UPL so that OpenDet can be trained in an end-to-end manner.
Tab.~\ref{tab:e2e_vs_finetune} shows that jointly optimizing UPL performs better than that of fine-tuning.

\noindent {\bf Open-RetinaNet.}
To further demonstrates the effectiveness of Open-RetinaNet,
we report more results in Tab.~\ref{tab:open_retinanet_more},
where Open-RetinaNet shows substantial improvements on WI, AOSE and~\APU, and achieves comparable performance on~\mAPK.

\noindent {\bf Vision transformer as backbone.}
We find the detector with vision transformer, \emph{e.g.}, Swin Transformer~\cite{liu2021swin} is a stronger baseline for OSOD.
As shown in Tab.~\ref{tab:swin_backbone}, models with a Swin-T backbone significantly suppress their ResNet counterparts.

\noindent {\bf Speed and computation.}
In the training stage, OpenDet only increases 14\% (1.4h \emph{vs.} 1.2h) training time and 1.2\% (2424Mb \emph{vs.} 2395Mb) memory usage.
In the testing phase, as we only add the unknown class to the classifier, OpenDet keeps similar running speed and computation with FR-CNN.

\begin{table}[t]
    \input{tables/appendix/upl_joint_vs_funetuning.tex}
    \caption{{\bf End-to-end \emph{vs.} fine-tune in UPL.}
    {\bf End-to-end:} we jointly optimize UPL and other modules in OpenDet. 
    {\bf Fine-tune:} we pretrain a model without UPL, and optimize UPL in the fine-tuning stage.
    }
    % \vspace{-2mm}
    \label{tab:e2e_vs_finetune}
    \end{table}

\begin{table}[t]
    \input{tables/appendix/voc_coco_a_retinanet.tex}
    \vspace{-1mm}
    \caption{{\bf Open-RetinaNet on more datasets.}}
    % \vspace{-3mm}
    \label{tab:open_retinanet_more}
    \end{table}

\begin{table}[t]
    \input{tables/appendix/swin_backbone.tex}
    \vspace{-1mm}
    \caption{{\bf Comparisons of different backbones}, \emph{i.e.}, ResNet-50~\cite{he2016resnet} and Swin-T~\cite{liu2021swin}.}
    % \vspace{-2mm}
    \label{tab:swin_backbone}
    \end{table}

\section{Comparison with ORE~\cite{joseph2021towards}}
\noindent {\bf Implementation details.}
The original ORE adopted a R50-C4 FR-CNN framework, and train the model with 8 epochs.
For fair comparisons, we replace the R50-C4 architecture with R50-FPN, and train all models with 3$\times$ schedule.
Besides, as discussed in these issues\footnote[1]{\href{https://github.com/JosephKJ/OWOD/issues?q=is:issue+cannot+reproduce}{https://github.com/JosephKJ/OWOD/issues?q=cannot+reproduce}},
we report our re-implemented results when comparing with ORE in an open world object detection task (see Tab.~\ref{tab:owod_t1}).

\noindent {\bf Analysis of ORE.} To learn the energy-based unknown identifier (Sec 4.3 in~\cite{joseph2021towards}), ORE requires an additional validation set with the annotations of unknown classes.
We notice that ORE continues to train on the validation set, so that the model can leverage the information of unknown classes.
In Tab.~\ref{tab:ore}, we find ORE without training on valset (\emph{i.e.}, froze parameters) obtains a rather lower \mAPK~(53.96 \emph{vs.} 58.45), and large amounts of known examples are misclassified to unknown.
In contrast, OpenDet outperforms ORE without using the information of unknown classes.

\begin{table}[t]
    \input{tables/appendix/ore.tex}
    \vspace{-1mm}
    \caption{{\bf Comparison with ORE~\cite{joseph2021towards}.}
    The row with \textcolor{gray}{gray} background is reported in our main paper.
    }
    % \vspace{-2mm}
    \label{tab:ore}
    \end{table}

\noindent {\bf Results on open world object detection.}
We also compare OpenDet with ORE in the task1 of open world object detection.
As shown in Tab.~\ref{tab:owod_t1}, without accessing open-set data in the training set or validation set,
OpenDet outperforms FR-CNN and ORE by a large margin and achieves comparable results with the Oracle.

\begin{table}[t]
    \input{tables/appendix/OWOD_task1.tex}
    \vspace{-1mm}
    \caption{{\bf Results on open world object detection~\cite{joseph2021towards}.}}
    % \vspace{-3mm}
    \label{tab:owod_t1}
    \end{table}

\section{Comparison with DS~\cite{miller2018dropout}}
% how to generate APU with entropy test
% extend entropy to our method
% discribe that we use entropy thresholding.
\noindent {\bf Implementation details.} DS averages multiple runs of a dropout-enabled model to produce more confident preditions.
As DS has no public implementation, we implement it based on the FR-CNN~\cite{ren2017faster} framework.
Specifically, we insert a dropout layer to the second-last layer of the classification branch in R-CNN, and set the dropout probability to 0.5.
Previous works~\cite{dhamija2020overlooked,joseph2021towards} indicate that DS works even worse than the baseline method;
we show it is effective as long as we remove the dropout layer during training, \emph{i.e.}, we only use the dropout layer in the testing phase.
Besides, original DS can only tell what is known, but do not have a metric for the unknown (\emph{e.g.}, the unknown probability in OpenDet).
We give DS the ability to identify unknown by entropy thresholding~\cite{hendrycks2016baseline}.
In detail, we define proposals with the entropy larger than a threshold (\emph{i.e.}, 0.25) as unknown.

\noindent {\bf DS with different \#runs.} DS requires multiple runs for a given image. We report DS with different number of \#runs in Tab.~\ref{tab:dropout_sampling}.
By increasing \#runs, DS shows substantial improvements on AOSE and \mAPK, while the performance on WI becomes worse.
We report DS with 30 \#runs in our main paper, which is consistent with its original paper~\cite{miller2018dropout}.
\vspace{-3mm}
\begin{table}[t]
    \input{tables/appendix/dropout_sampling.tex}
    \caption{{\bf Comparison with DS~\cite{miller2018dropout}.} 
    \#runs denotes the number of runs used for ensemble.
    The row with \textcolor{gray}{gray} background is reported in our main paper.
    }
    \vspace{-3mm}
    \label{tab:dropout_sampling}
    \end{table}

\section{More Qualitative Results.}
Fig.~\ref{fig:more_qualitative_results} gives more qualitative comparisons between the baseline method and OpenDet.
OpenDet can recall unknown objects from known classes and the "background".
Besides, we also give two failure cases in Fig.~\ref{fig:failure_cases}.
{\bf (a)} We find OpenDet performs poorly in some scenes with dense objects, \emph{e.g.}, images with lots of \texttt{person}.
{\bf (b)} OpenDet classifies "real" background to the \texttt{unknown} class.

\begin{figure}[h]
    \includegraphics[width=\linewidth]{figures/appendix/failure_cases.pdf}
    \vspace{-5mm}
    \caption{{\bf Failure cases.}}
    \label{fig:failure_cases}
\end{figure}

\begin{figure*}[h!]
    \centering
    \includegraphics[width=0.95\textwidth]{figures/appendix/more_qualitative_results.pdf}
    \caption{{\bf More qualitative comparisons} between the baseline and OpenDet.}
    \label{fig:more_qualitative_results}
\end{figure*}
